# Supplementary material for: Resonance-enhanced multiphoton ionization in the x-ray regime
Source: arXiv:2110.08145 source file (2021-11-05)
Supplement: Supplementary file 1 [file Ar_XFEL_supplement.pdf]

# Supplement: Resonance-enhanced multiphoton ionization in the x-ray regime


Aaron C. LaForge,[1] Sang-Kil Son (손상길),[2,3] Debadarshini Mishra,[1] Markus Ilchen,[4,5] Stephen Duncanson,[1] Eemeli Eronen,[6] Edwin Kukk,[6] Stanislaw Wirok-Stoletow,[2,7] Daria Kolbasova,[2,7] Peter Walter,[8] Rebecca Boll,[4] Alberto De Fanis,[4] Michael Meyer,[4] Yevheniy Ovcharenko,[4] Daniel Rivas,[4] Philipp Schmidt,[4] Sergey Usenko,[4] Robin Santra,[2,3,7] and Nora Berrah[1]

[1]*Department of Physics, University of Connecticut, Storrs, Connecticut 06269, USA*
[2]*Center for Free-Electron Laser Science CFEL, Deutsches Elektronen-Synchrotron DESY, 22607 Hamburg, Germany*
[3]*The Hamburg Centre for Ultrafast Imaging, 22761 Hamburg, Germany*
[4]*European XFEL GmbH, 22869 Schenefeld, Germany*
[5]*Institut für Physik und CINSaT, Universität Kassel, 34132 Kassel, Germany*
[6]*Department of Physics and Astronomy, University of Turku, 20014 Turku, Finland*
[7]*Department of Physics, Universität Hamburg, 22607 Hamburg, Germany*
[8]*Linac Coherent Light Source, SLAC National Accelerator Laboratory, Menlo Park, California 94025, USA*


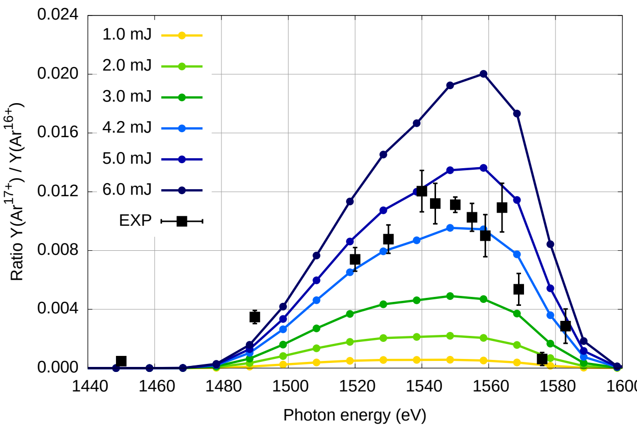


Figure S1. Dependence of the resonance profile on the FEL pulse energy. A pulse length of 10 fs FWHM, a second harmonic contribution of 0.2%, and an FEL bandwidth of 1% are fixed in calculations. By modeling with xcalib [39], the peak fluence (corresponds to a pulse energy of 6.0 mJ) at 1550 eV was calibrated to be $1.6\times10^{12}$ ph/$\mu$m$^2$ and $2.3\times10^{12}$ ph/$\mu$m$^2$ by measuring the ion yields of Ne and Ar (charge states less than +16) as reference gases, respectively, assuming a single Gaussian spatial fluence distribution in the interaction region. If we assume a focal area of 1.5 $\mu$m$\times$1.5 $\mu$m, the corresponding beamline transmissions are 17.1% (Ne) and 23.8% (Ar). Since the calibration determines only the ratio between the transmission, measured to be about 70% at these photon energies, and the focal area, the simulations would indicate a somewhat larger focal area or a non-Gaussian beam profile. Note that this pulse-energy dependence can be considered equivalently as the dependence on peak fluence or transmission.

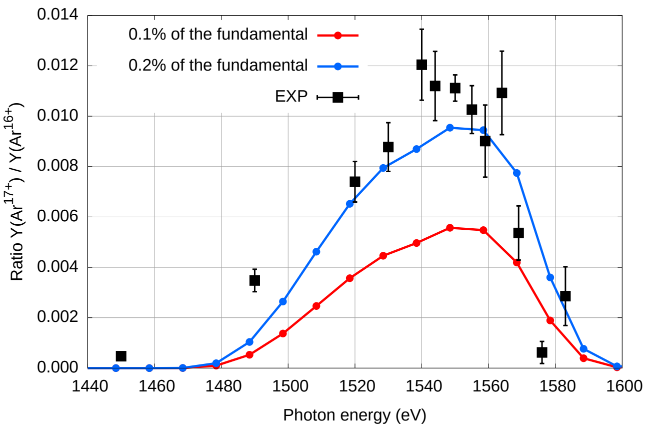


Figure S2. Dependence of the resonance profile on the second harmonic contribution. A pulse energy of 4.2 mJ is fixed and other FEL beam parameters (except for the second harmonic contribution) are the same as used in Fig. S1. The contribution of the second harmonic can strongly vary between experiments, depending on the FEL beam parameters and electron energy.

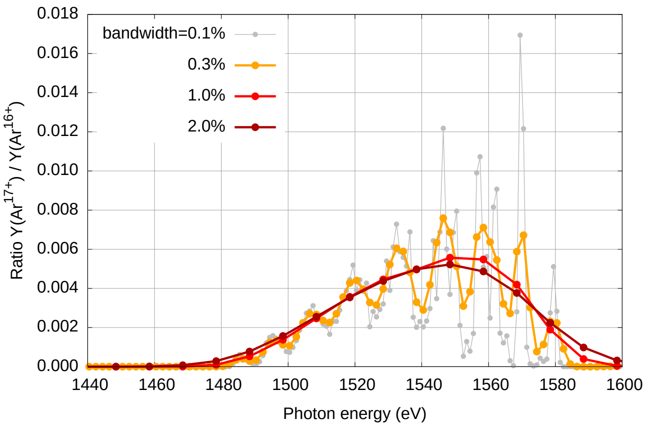


Figure S3. Dependence of the resonance profile on the FEL energy bandwidth. Note that a second harmonic contribution of 0.1% is used. The other FEL beam parameters (except for the FEL bandwidth) are the same as used in Fig. S2.

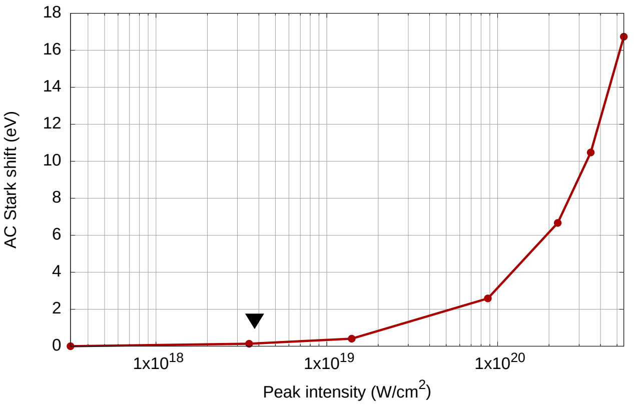


Figure S4. AC Stark shift for the two-photon resonant excitation of $Ar^{16+}$ as a function of peak intensity, calculated using the time-dependent configuration interaction singles (TDCIS) method [41]. Within TDCIS, the two-photon resonance lies at 1557.7 eV in the limit of low intensity and, through the AC Stark effect, is blue-shifted as the peak intensity increases. The shift is negligible for intensities below the highest value estimated in our experiment ($3.8\times10^{18}$ W/cm$^2$, marked with the down-pointing triangle).

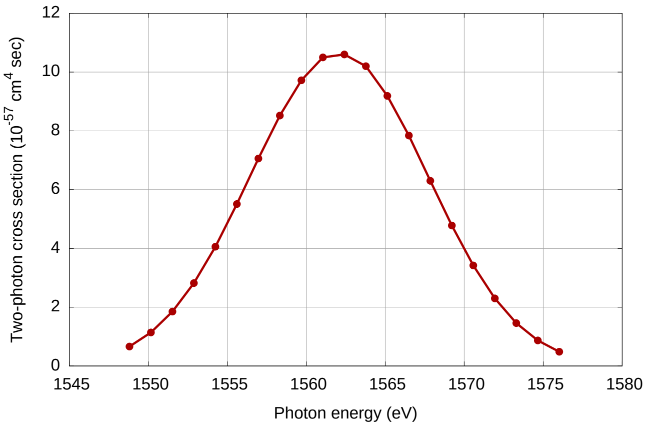


Figure S5. Nonsequential (direct) two-photon resonant excitation cross section for the $1s^2 \rightarrow 1s2s$ transition of $Ar^{16+}$ as a function of photon energy. The results have been horizontally shifted by the difference between the TDCIS resonance energy (1557.7 eV) and half of the one-photon transition energy in the literature (1562.3 eV) [45].

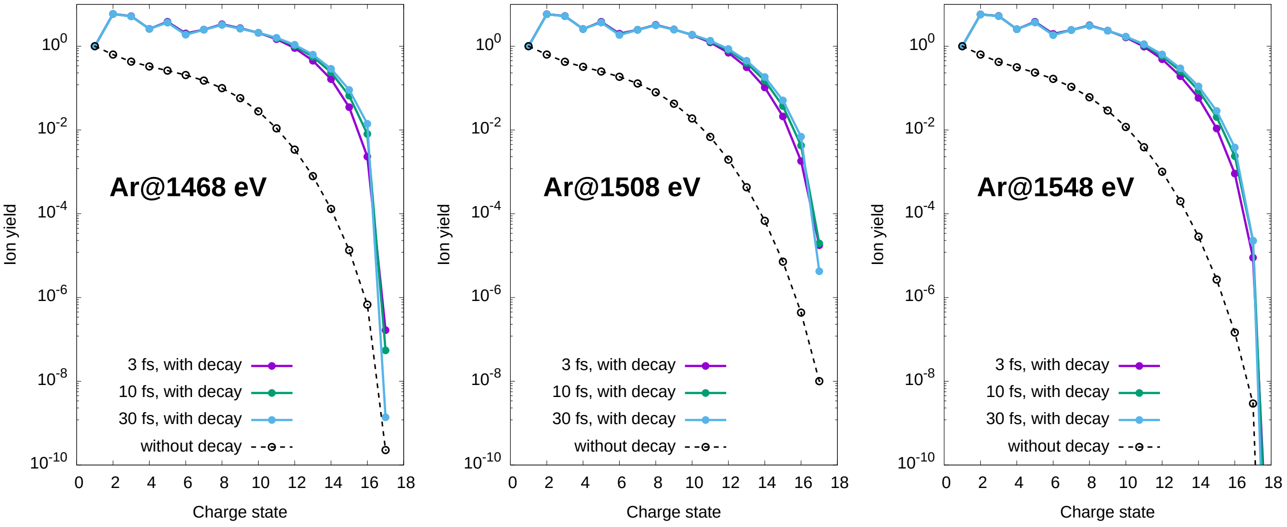


Figure S6. Calculated charge-state distributions (CSDs) of Ar for different photon energies with and without Auger-Meitner and fluorescence decay. In the latter calculations, we excluded all decay channels in the calculation to demonstrate the importance of ultrafast decay in the overall ionization process. For decay included, three different pulse lengths are plotted. For decay excluded, however, there is no pulse-length dependence. Furthermore, the ion yields of the high charge states are strongly suppressed. A pulse energy of 4.2 mJ is fixed and other FEL beam parameters are the same as used in Fig. S1. The CSDs are scaled to keep the same ion yield of +1.

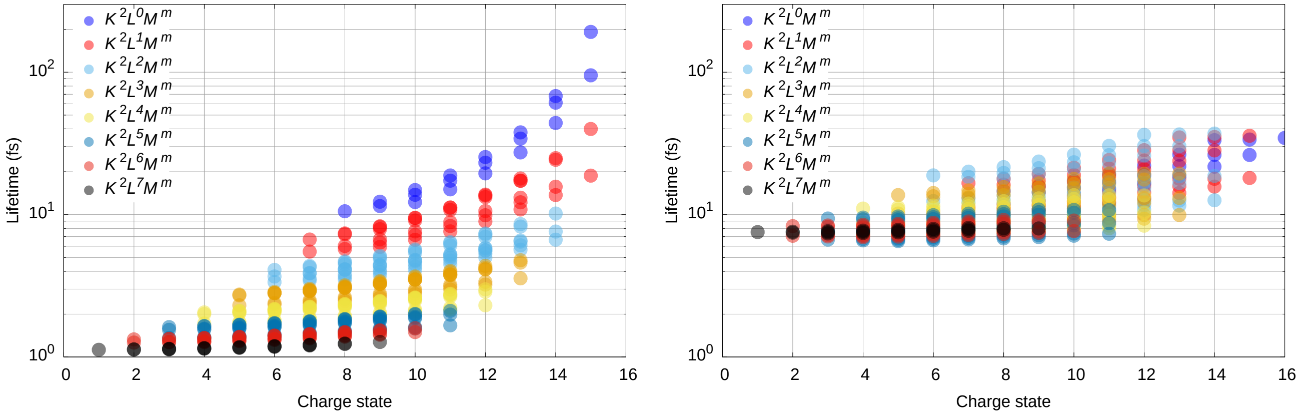


(a) Auger-Meitner

(b) Fluorescence

Figure S7. Lifetimes of (a) Auger-Meitner [28] and (b) fluorescence decay for a $1s$ vacancy as a function of charge state, calculated using XATOM. They are calculated for individual electron configurations and grouped with multiple colors, according to the occupation number in the $L$ shell, where $K^2L^lM^m$ indicates the electron configuration before the resonant excitation of $1s \to 2p$. Note that fluorescence lifetimes are comparable with Auger-Meitner lifetimes for highly charged ions.

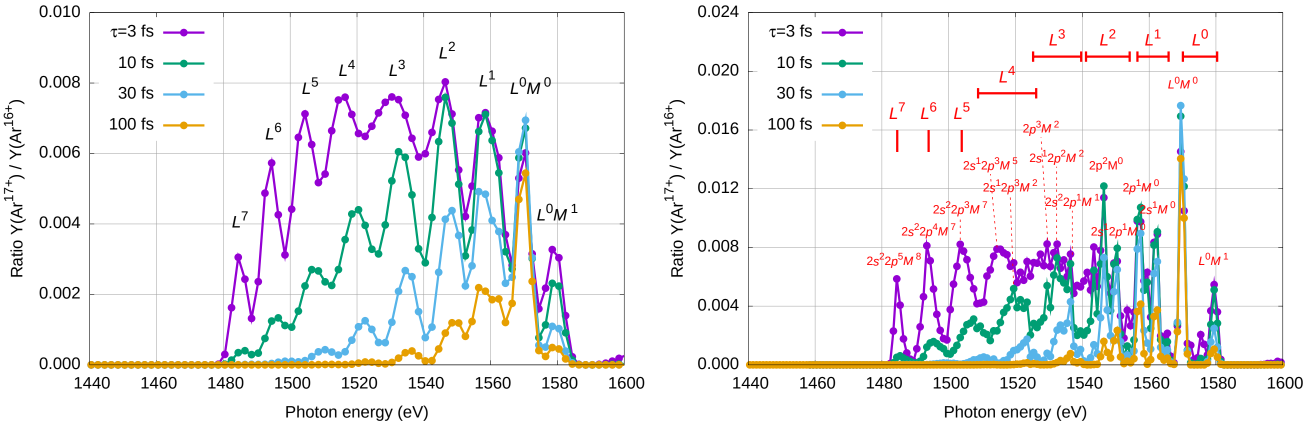


(a) FEL bandwidth of 0.3%

(b) FEL bandwidth of 0.1%

Figure S8. Dependence of the resonance profile on the pulse length with narrower FEL bandwidths. Note that a second harmonic contribution of 0.1% is used. The pulse length is varied and two narrower bandwidths of (a) 0.3% and (b) 0.1% are employed. The other FEL beam parameters are the same as used in Fig. S2. As the FEL bandwidth becomes narrower, individual super-configurations with an occupation number of the $L$ shell (the $M$ shell for $L^0$) and some of the electron configurations could be resolved as shown with the (a) 0.3%- and (b) 0.1%-bandwidths, respectively.
